# Supplementary material for: A low-cost PPG sensor-based empirical study on healthy aging based on changes in PPG morphology
Source: arXiv:2312.13404 source file (2023-12-20)
Supplement: Supplementary file 1 [file appendix.tex]

\section{Appendix A}

\textcolor{red}{
Derivative markers make an important feature class and are identified as consistent inflection points that intersect with the original PPG waveform. These markers represent important peaks and points in the derivative waveforms (VPG, APG, JPG, SPG) calculated from the PPG signal. 
Inflection points, where the direction of the waveform changes (from increasing to decreasing or vice versa), are considered as potential markers. The methodology likely involves analyzing the slope and curvature of the derivative waveforms to identify these points accurately.
The fourth derivative PPG allows for a more detailed assessment of microvascular dynamics, capturing subtle changes related to endothelial function, vascular compliance, and peripheral vascular resistance. These fine-grained variations can provide insights into the health and functioning of the microcirculation. These parameters might include specific characteristics of the waveform shape, amplitude, or temporal features that can provide further insights into cardiovascular dynamics.
Peak detection involves identifying specific peaks in the PPG, VPG, and APG waveforms using the derivative markers. The methodology employs these derivative markers as references to detect fiducial points associated with various peaks in the waveforms.
For example, in the PPG waveform, the onset, systolic, notch, and diastolic peaks are detected using the derivative information. The derivative markers provide information about the slopes and changes in the waveform, allowing for the identification of these specific peaks.
Similarly, in the VPG waveform, the u, v, and w peaks are detected using the derivative markers as references. In the APG waveform, peaks labeled as a, b, c, d, and e are detected by utilizing the derivative information. The peak detection process may involve applying thresholding techniques or using specific algorithms to enhance the detection of primary points in the waveforms. Additionally, the methodology may include filtering techniques or other preprocessing steps to improve the accuracy and reliability of peak detection.
By identifying and detecting these peaks in the PPG, VPG, and APG waveforms, the methodology aims to provide valuable insights into the cardiovascular characteristics and dynamics of the subjects under study. In this work, we implement the derivative marker method for peak detection \cite{ppg4derivatives}.
}

%List of 26 important features (out of 60 features) retained for classification and regression:
%Index(['a', 'b', 'c', 'd', 'e', 'AGI', 't_ab', 't_bc', 't_cd', 't_de', 't_ac','t_ad', 't_ae', 't_bd', 't_be', 't_ce', 'b-a', '(b-e)/a', '(c+d-b)/a','b - (d/a)', 'ab_slope', 'ac_slope', 'ad_slope', 'ae_slope', 'bc_slope','bd_slope', 'be_slope', 'cd_slope', 'ce_slope', 'de_slope', 'dist_mea','dist_std', 'dist_med', 'dist_mad', 'diff_mea', 'diff_std', 'diff_med','diff_mad', 'n_dist_mea', 'n_dist_std', 'n_dist_med', 'n_dist_mad','n_diff_mea', 'n_diff_std', 'n_diff_med', 'n_diff_mad', 'dist_mea_all','dist_std_all', 'dist_med_all', 'dist_mad_all', 'diff_mea_all','diff_std_all', 'diff_med_all', 'diff_mad_all', 'n_dist_mea_all','n_dist_std_all', 'n_dist_med_all', 'n_dist_mad_all', 'n_diff_mea_all','n_diff_std_all', 'n_diff_med_all', 'n_diff_mad_all', 'family','Smoking', 'spo2', 'Rbpm', 'height', 'weight', 'Gender', 'bmi'],dtype='object')
